# Supplementary material for: Extracting analytical one-loop amplitudes from numerical evaluations
Source: arXiv:1904.04067 ancillary file (2023-10-06)
Supplement: Supplementary file 1 [file tree.pdf]

$$\begin{aligned}
& \frac{-1i\langle 35\rangle^4[12]^3}{s_{345}[16]\langle 45\rangle\langle 34\rangle\langle 3|1+2|6]\langle 5|1+6|2]} + \\
& \frac{1i[24]^4\langle 56\rangle^3}{s_{234}\langle 16\rangle[23][34]\langle 1|2+3|4]\langle 5|1+6|2]} + \\
& \frac{1i\langle 3|1+2|4]^4}{\langle 12\rangle\langle 23\rangle[45][56]\langle 1|2+3|4]\langle 3|1+2|6]s_{123}}
\end{aligned}$$

$$\begin{aligned}
& \frac{1 i \langle 56 \rangle^3 [12]^3}{s_{123} [23] \langle 45 \rangle \langle 6 | 1+2 | 3 \rangle \langle 4 | 2+3 | 1 \rangle} + \\
& \frac{-1 i \langle 6 | 1+2 | 4 \rangle^4}{s_{345} \langle 16 \rangle [45] [34] \langle 12 \rangle \langle 6 | 1+2 | 3 \rangle \langle 2 | 1+6 | 5 \rangle} + \\
& \frac{1 i \langle 3 | 2+4 | 1 \rangle^4}{[16] \langle 23 \rangle \langle 34 \rangle [56] \langle 2 | 1+6 | 5 \rangle \langle 4 | 2+3 | 1 \rangle s_{234}}
\end{aligned}$$
