# Supplementary material for: Extracting analytical one-loop amplitudes from numerical evaluations
Source: arXiv:1904.04067 ancillary file (2023-10-06)
Supplement: Supplementary file 2 [file tree.pdf]

$$\frac{1i\langle 4|2+3|1\rangle^3}{[16]\langle 23\rangle\langle 34\rangle[56]\langle 2|1+6|5\rangle s_{234}} +$$

$$(123456 \rightarrow 321654)$$

$$\frac{1i[23]^3\langle 56\rangle^3}{\langle 16\rangle[34]\langle 1|2+3|4\rangle\langle 5|1+6|2\rangle s_{234}} +$$

$$(123456 \rightarrow 321654) +$$

$$\frac{1is_{123}^3}{\langle 12\rangle\langle 23\rangle[45][56]\langle 1|2+3|4\rangle\langle 3|1+2|6\rangle}$$

$$\frac{1i[12]\langle 45\rangle\langle 4|2+3|1|^2}{[16]\langle 23\rangle\langle 34\rangle[56]s_{234}s_{345}} +$$

$$(123456 \rightarrow 321654) +$$

$$\frac{1i\langle 4|2+3|1\rangle\langle 6|1+2|3\rangle s_{123}}{\langle 12\rangle\langle 23\rangle[45][56]s_{234}s_{345}}$$
